# Supplementary material for: Exploring PROTAC cooperativity with coarse-grained alchemical methods
Source: arXiv:2208.06446 source file (2022-11-17)

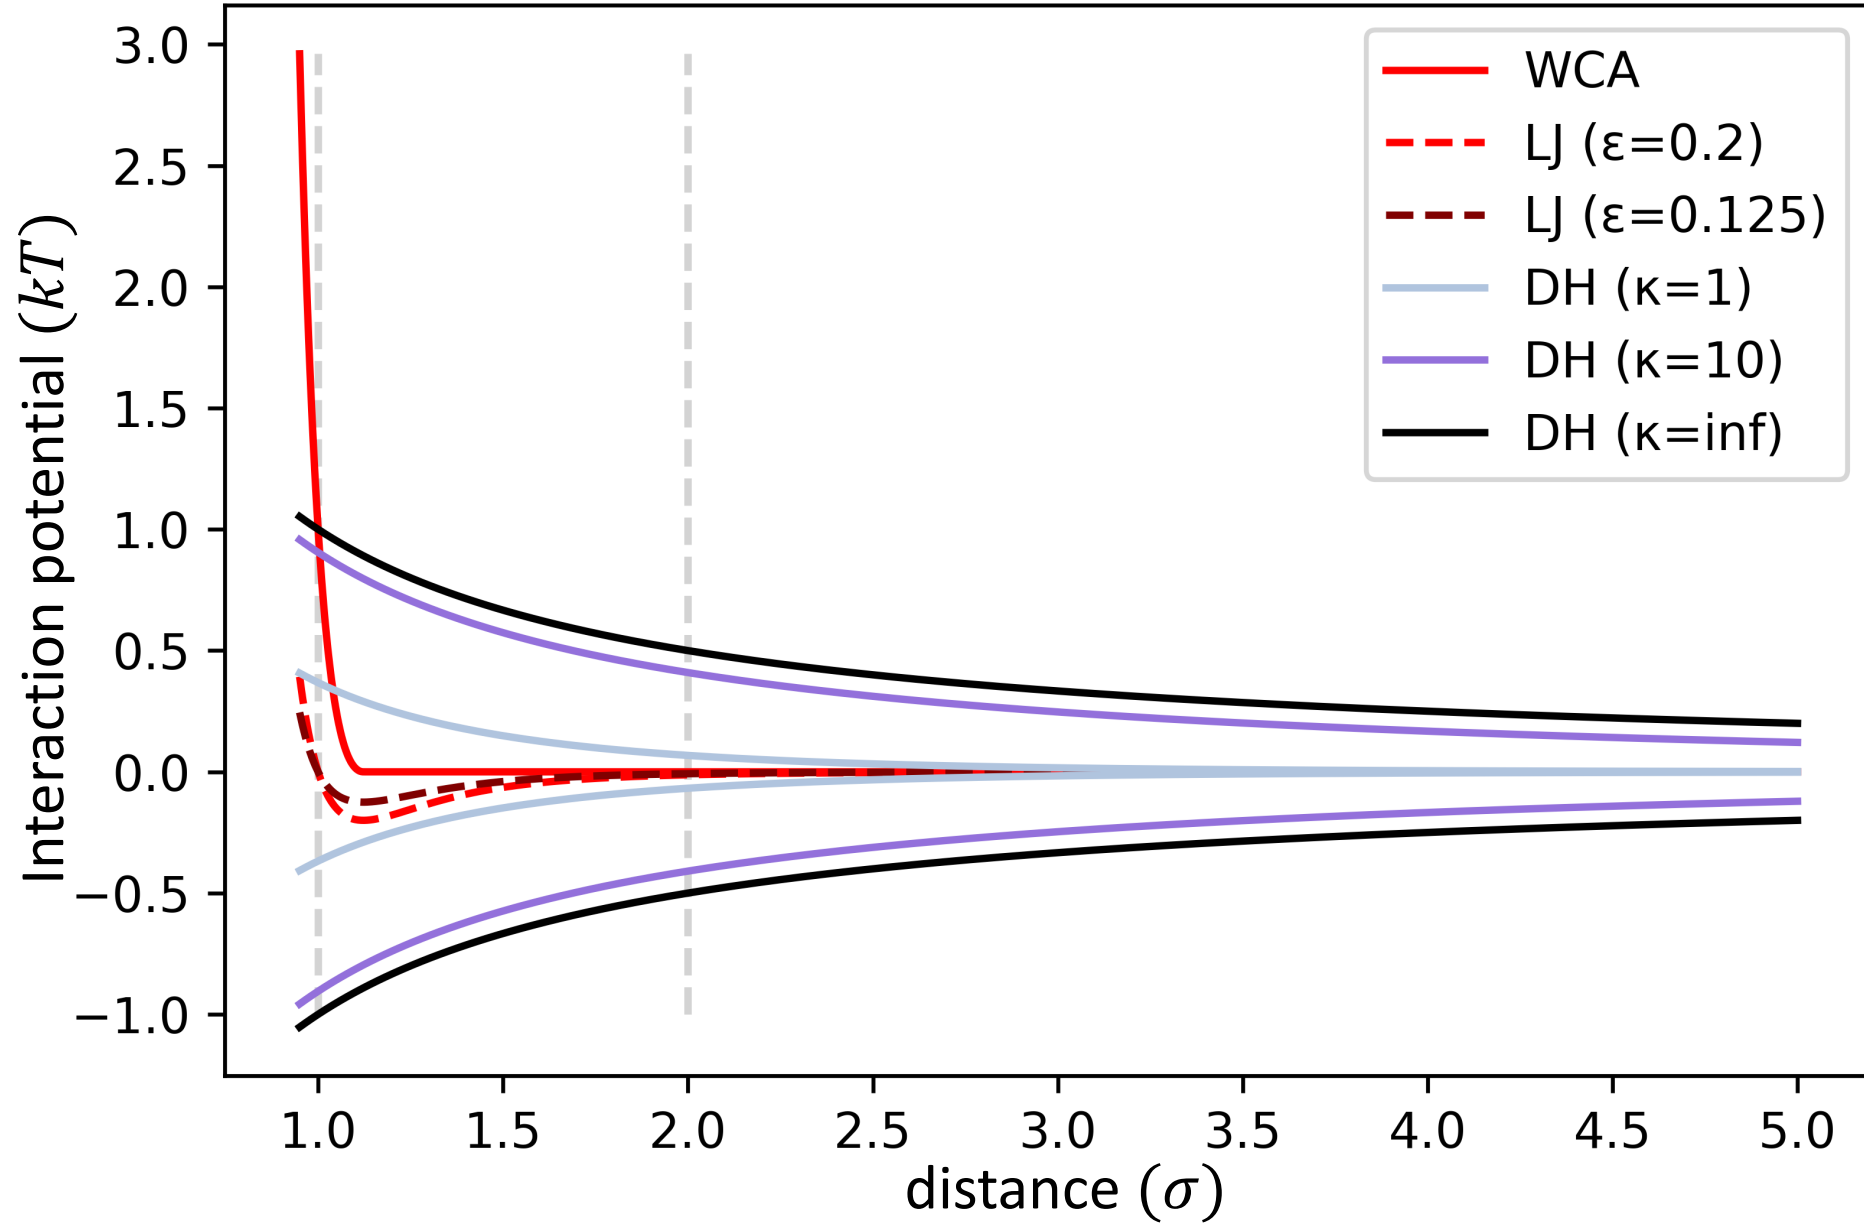

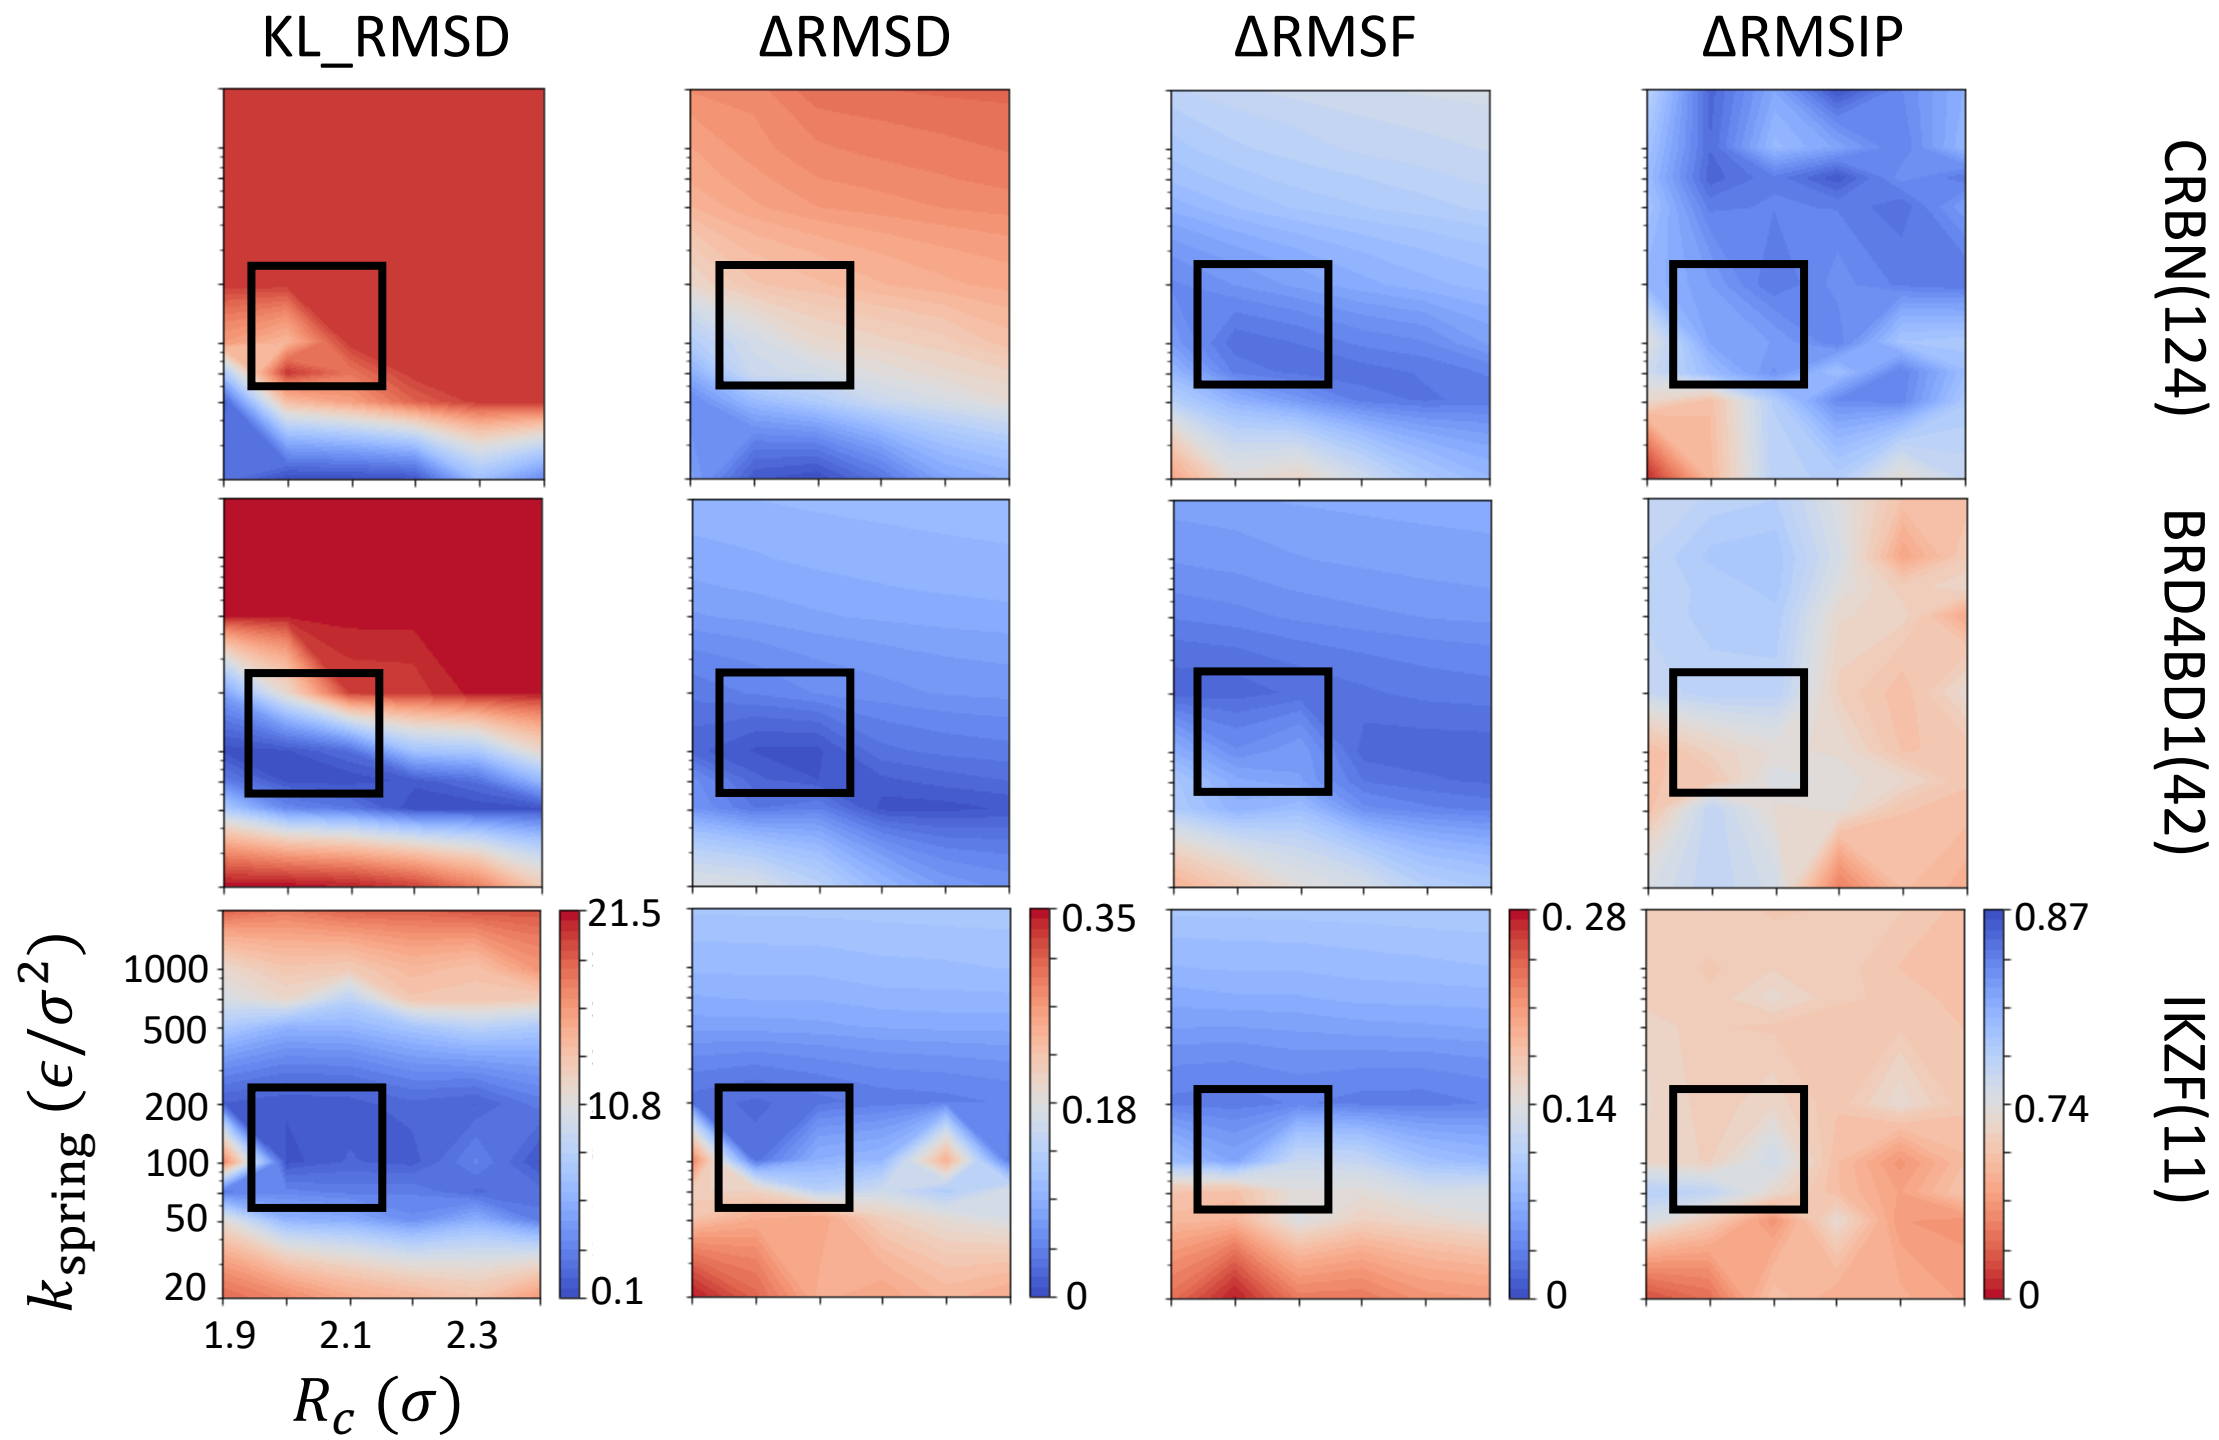

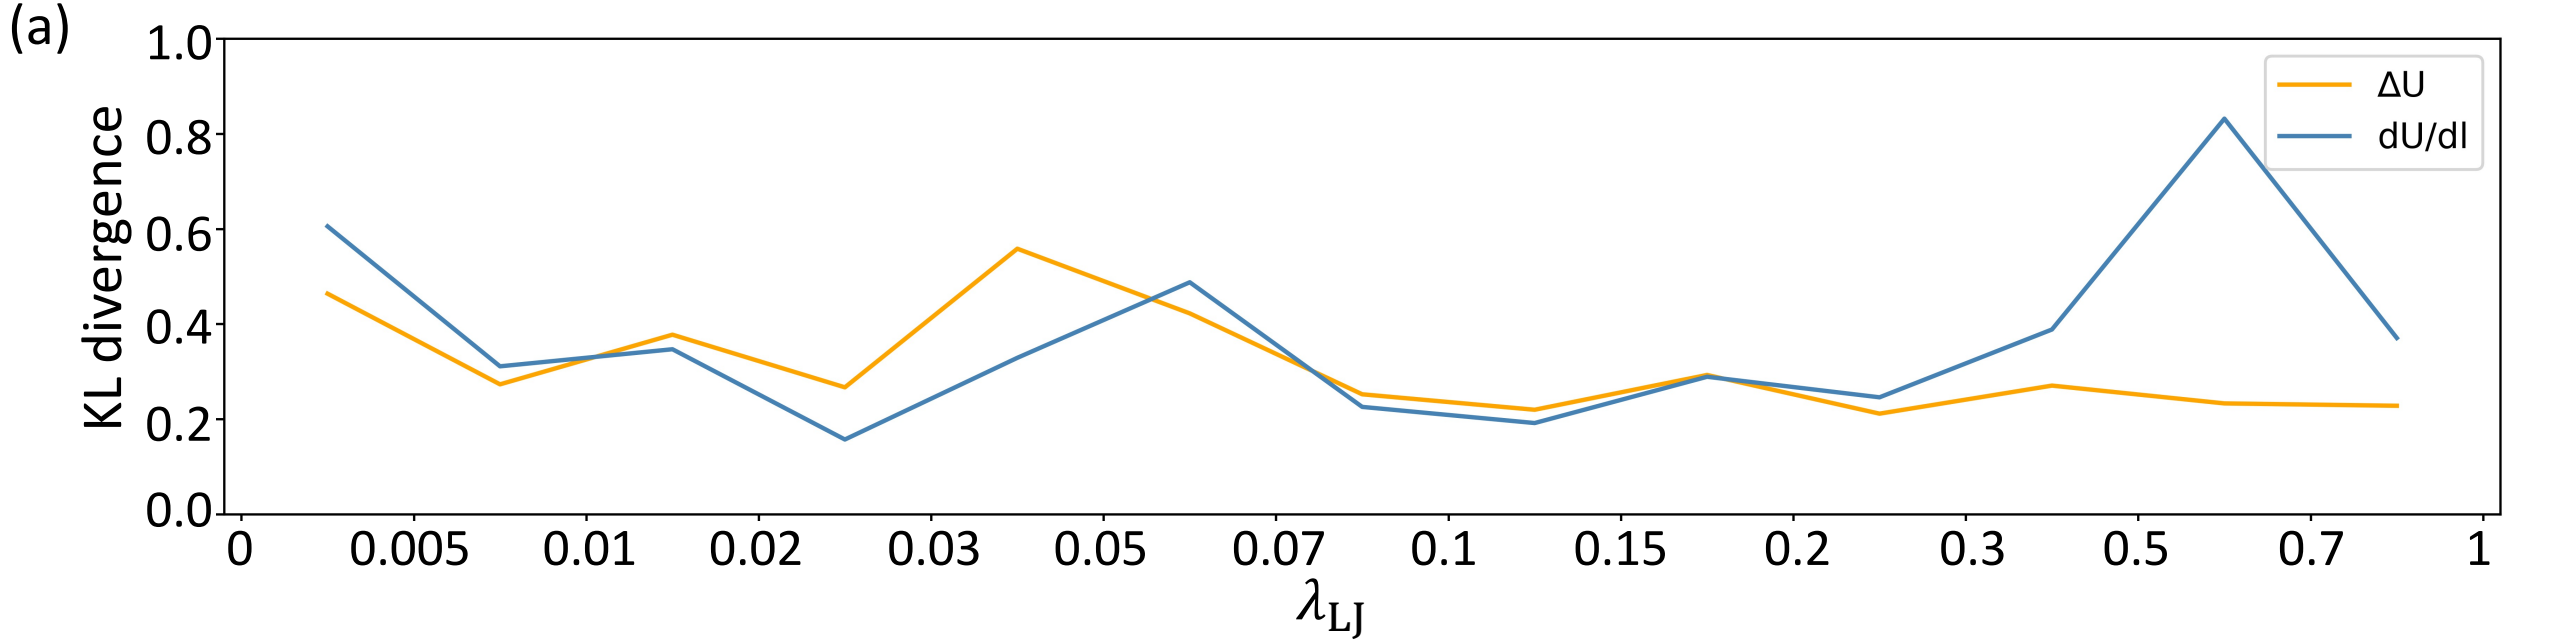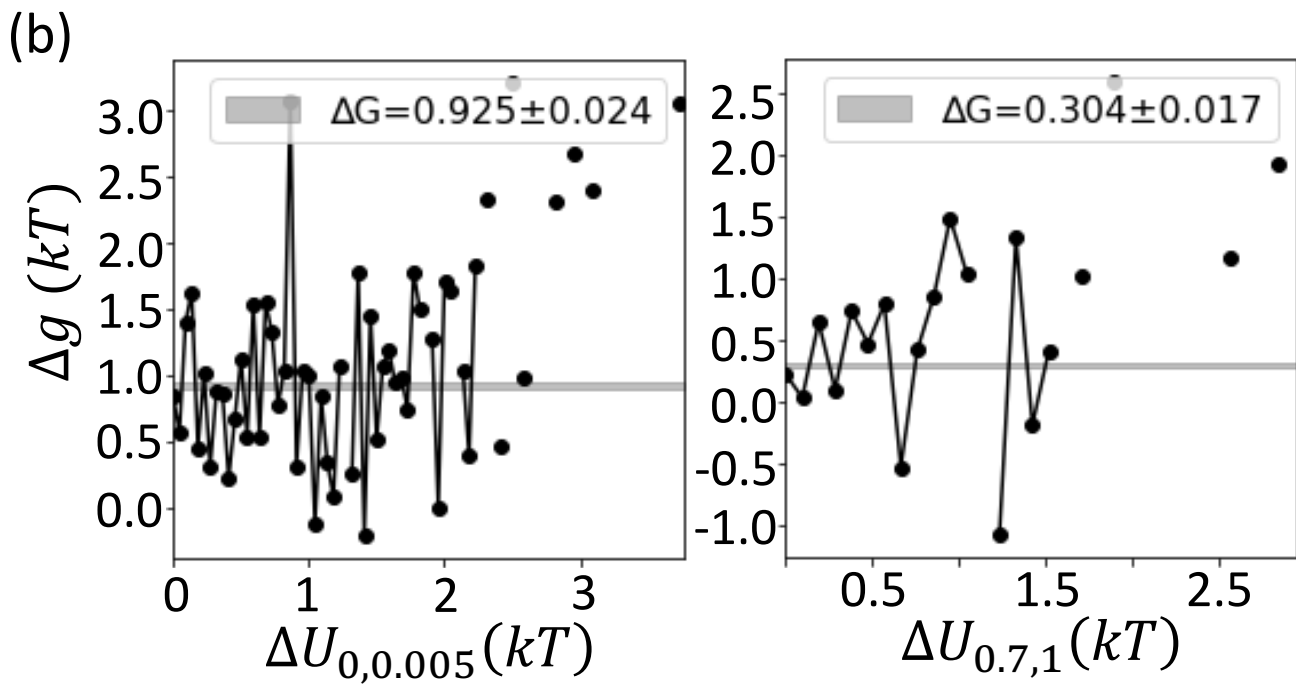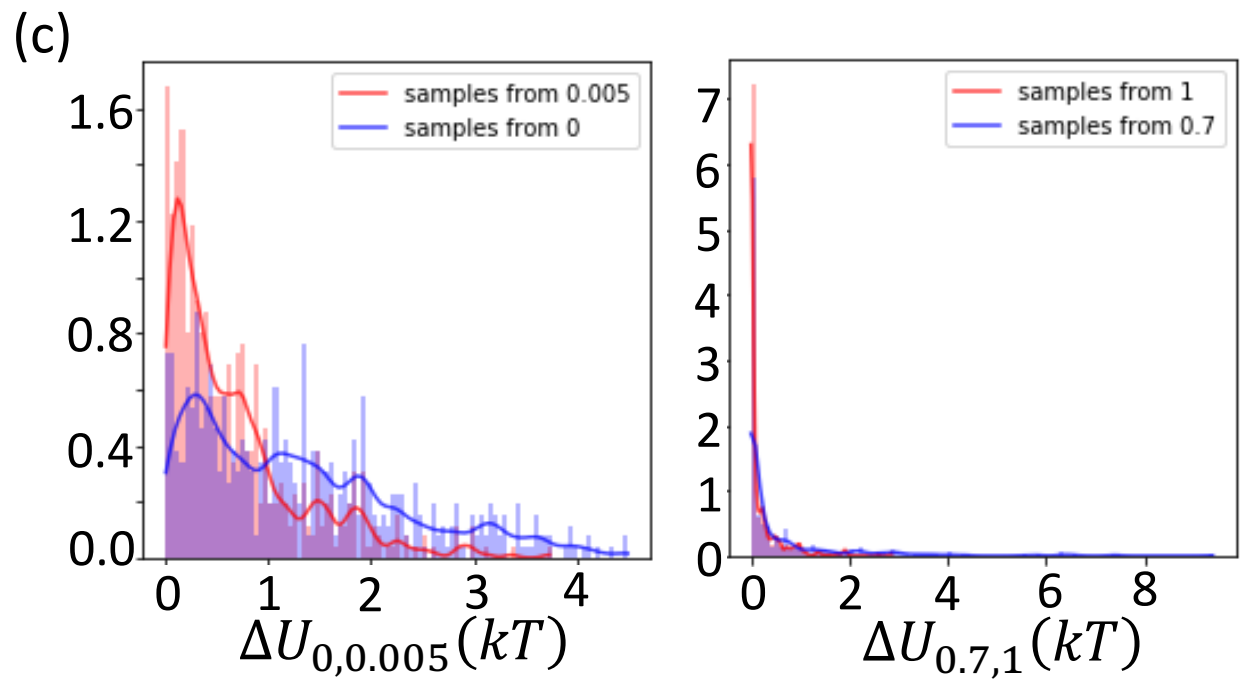

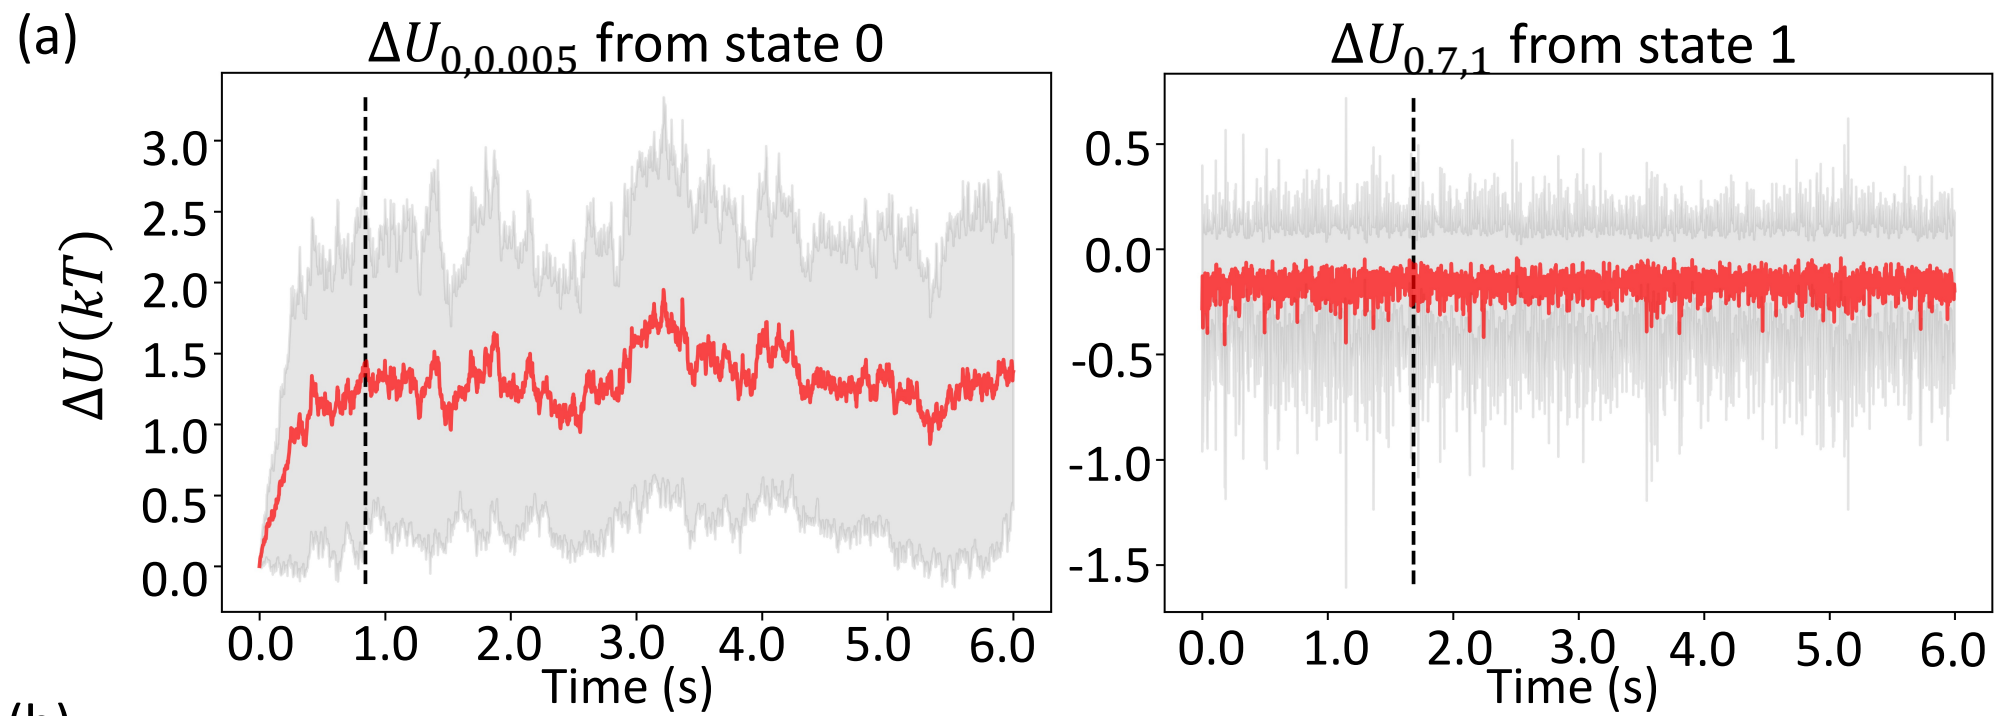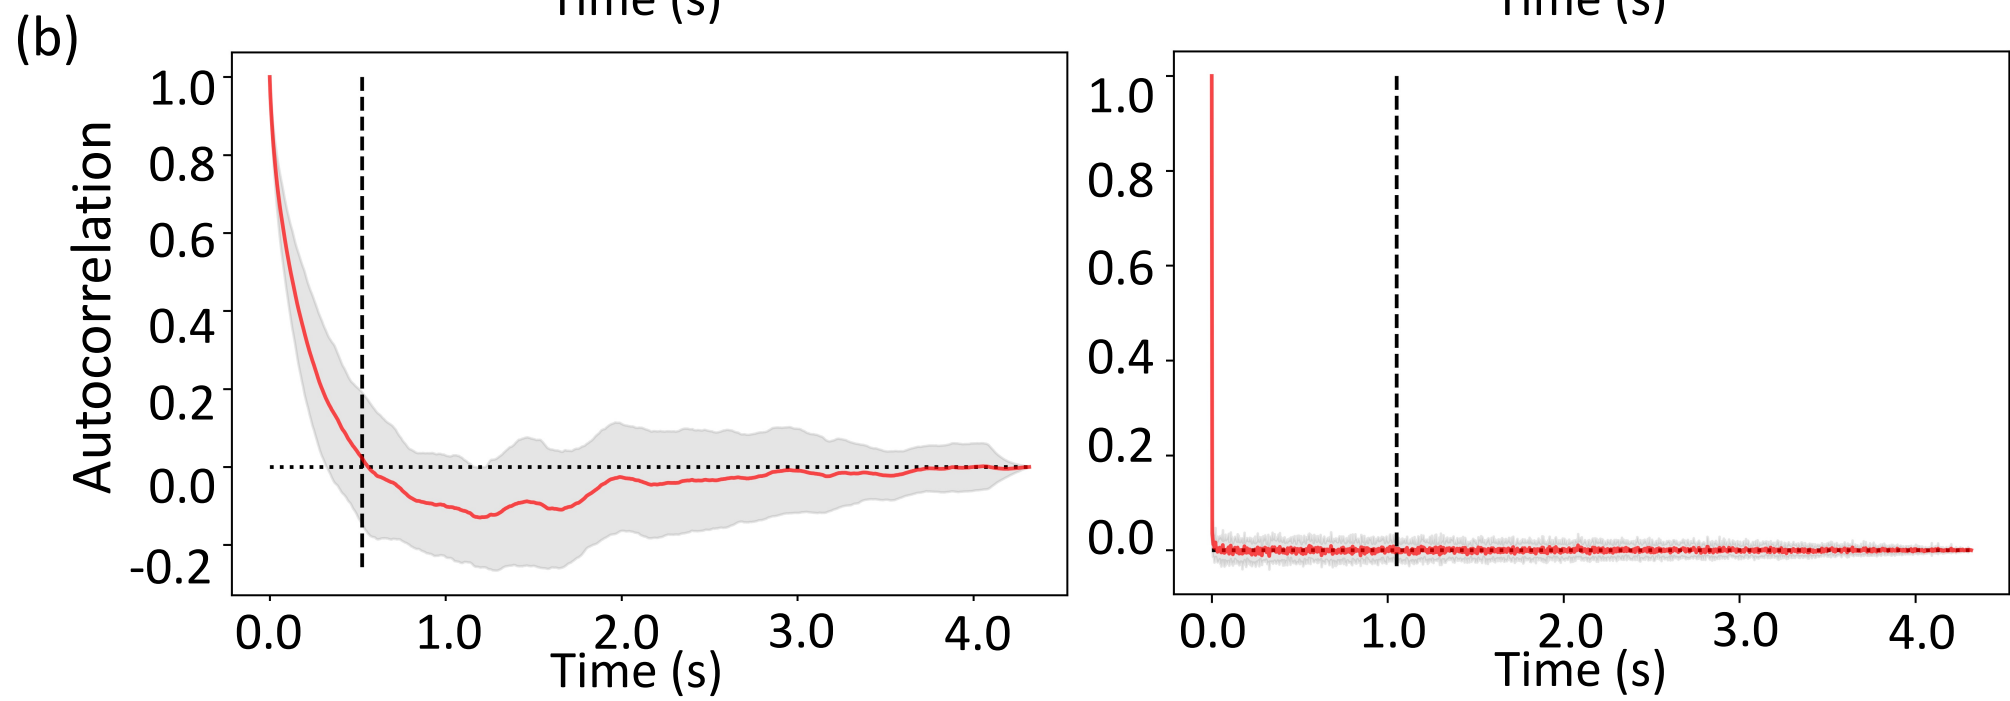

(a)

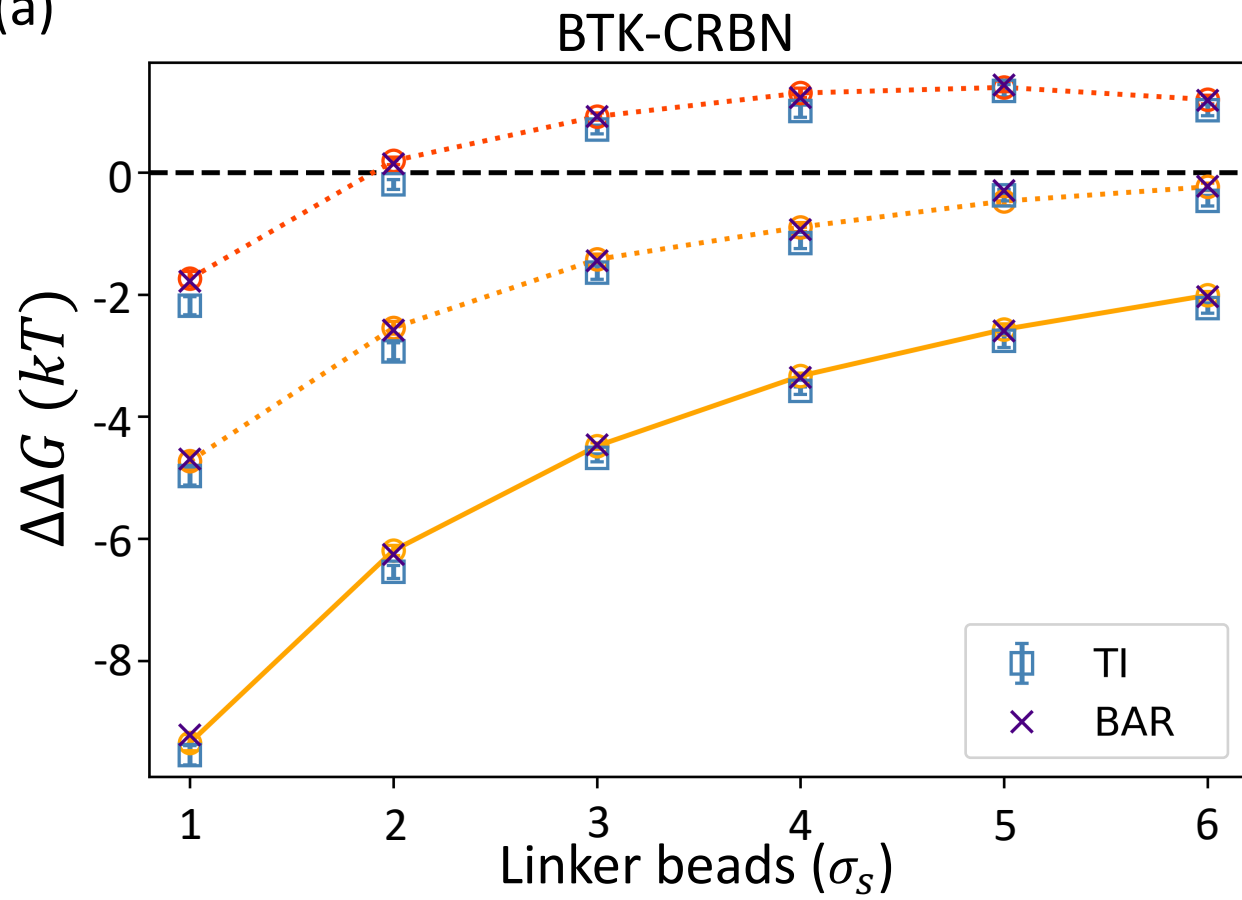

(b)

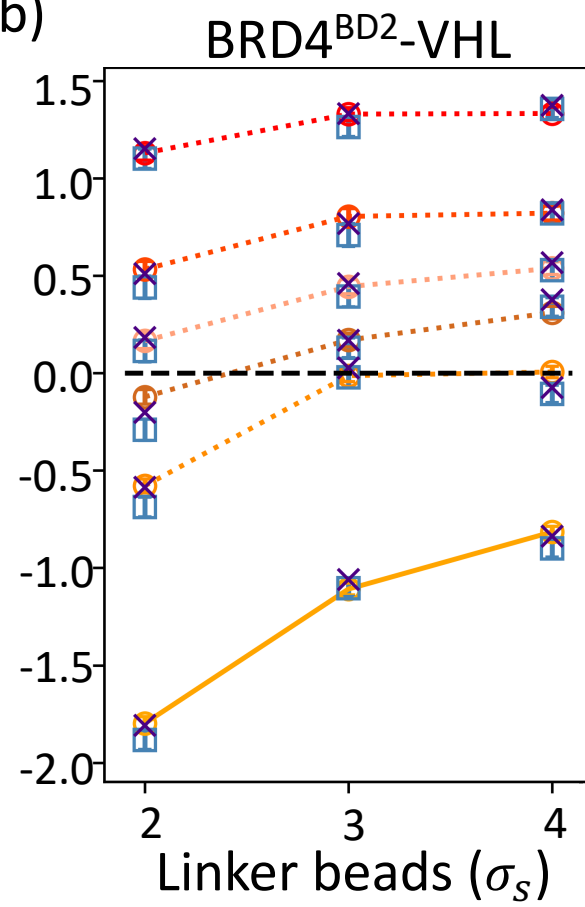

(a)

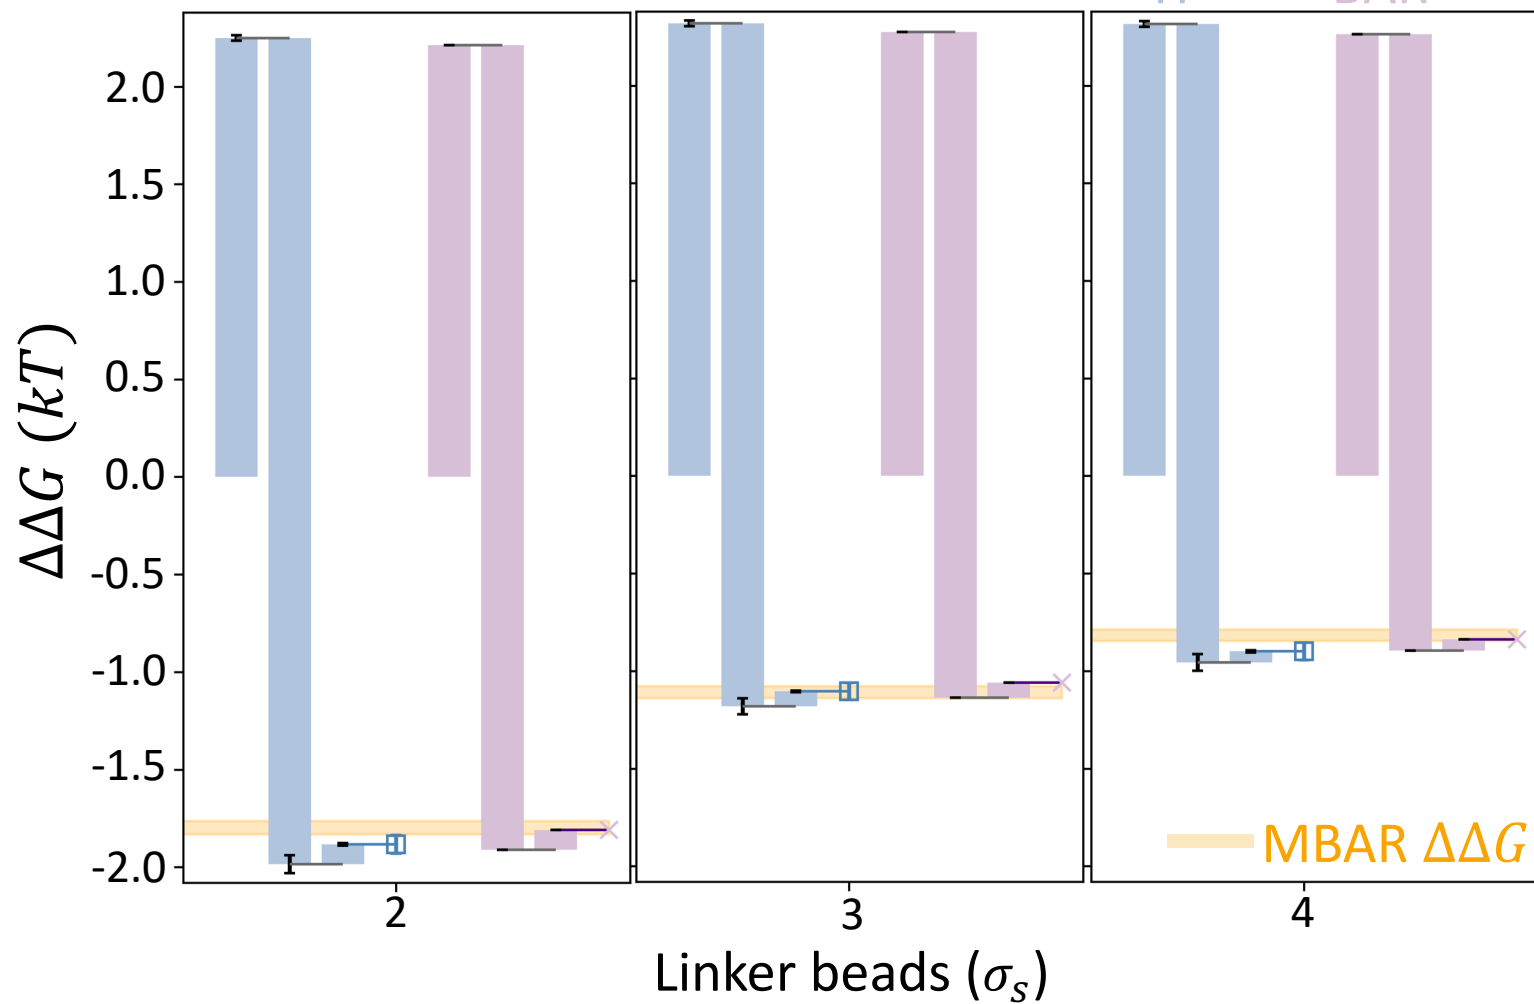

(b)

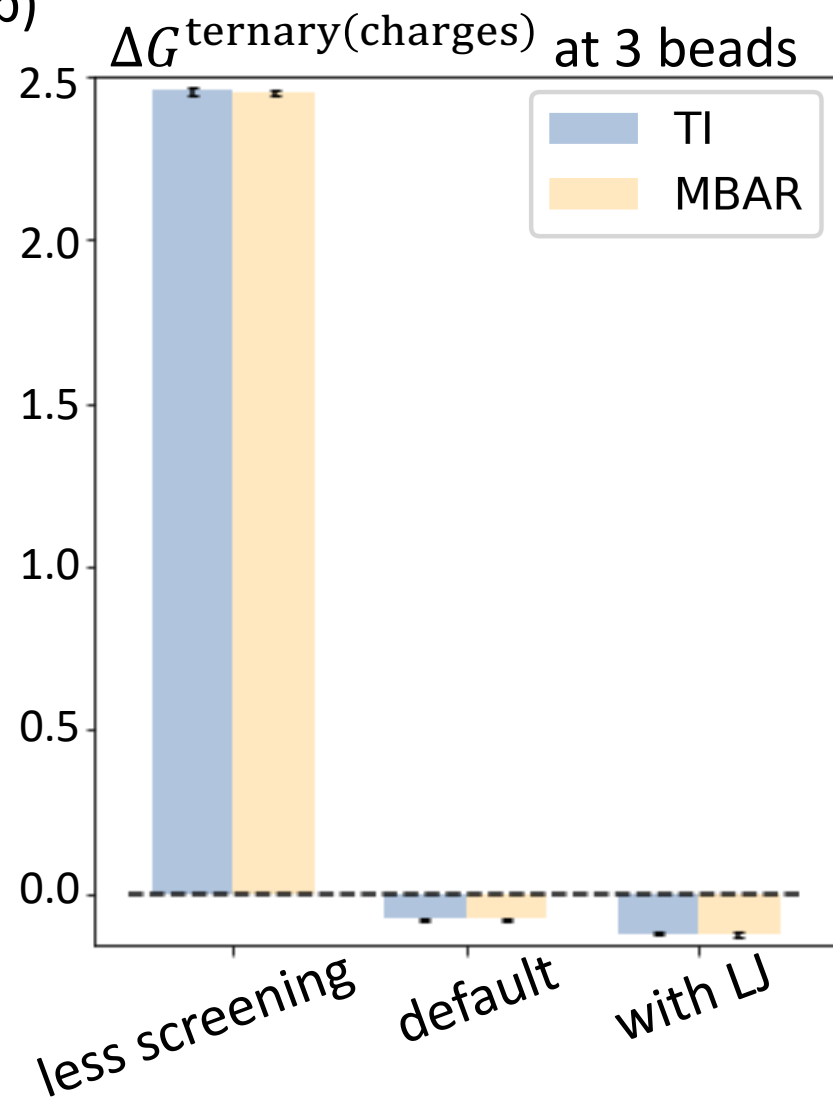

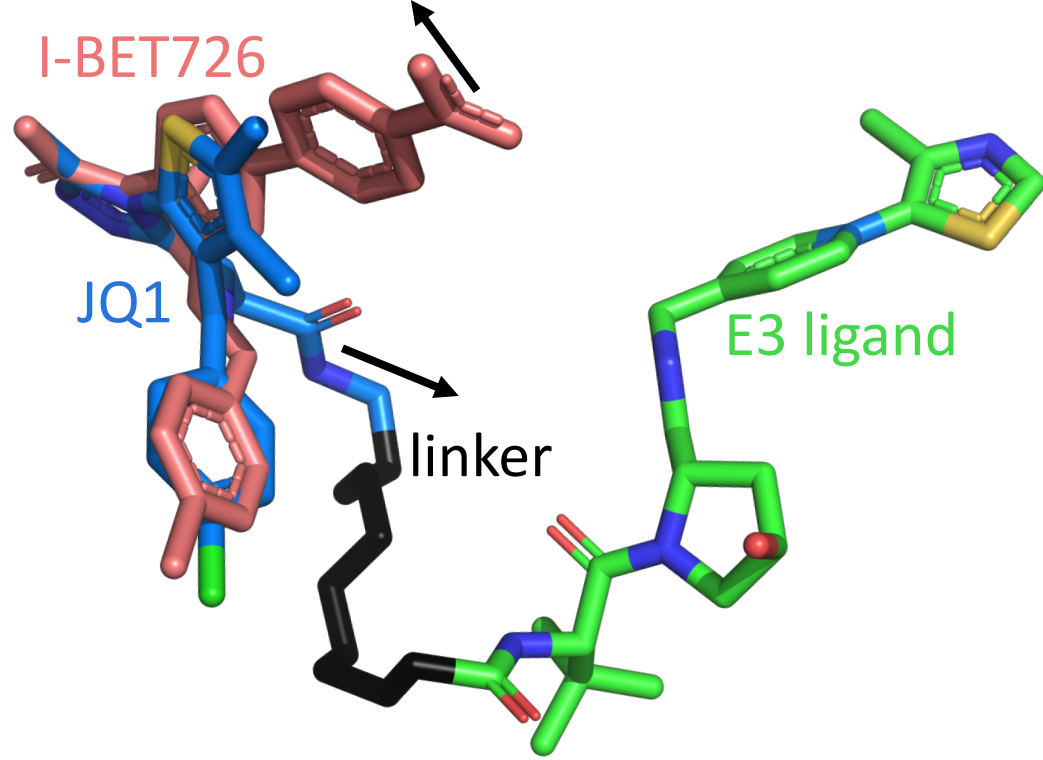

Supplement: Supplementary file 1 [file SI_figs.pdf]
